# Supplementary material for: Highly Sensitive, Fast Graphene Photodetector with Responsivity $>10^6$ A/W Using Floating Quantum Well Gate
Source: arXiv:1908.06924 source file (2019-08-19)
Supplement: Supplementary file 1 [file SI.pdf]

Supporting Information:

Highly Sensitive, Fast Graphene  
Photodetector with Responsivity  $> 10^6$  A/W  
Using Floating Quantum Well Gate

Krishna Murali, Nithin Abraham, Sarthak Das, Sangeeth Kallatt, and Kausik  
Majumdar\*

*Department of Electrical Communication Engineering,  
Indian Institute of Science, Bangalore 560012, India*

E-mail: [kausikm@iisc.ac.in](mailto:kausikm@iisc.ac.in)

## S1. Characterization of photodetector D2

In this section we describe the performance of another few-layer graphene (FLG)/2L-WS<sub>2</sub>/1L-MoS<sub>2</sub> vertical heterojunction photodetector (D2). Optical images of the different fabrication steps are shown in Figure S1 (a). The junction area of D2 is 14  $\mu\text{m}^2$ . The  $I_d$ - $V_g$  characteristics of the top few layer graphene shows a negative Dirac voltage, similar to the photodetector D1 presented in the main text. We thus expect a negative photocurrent from D2 as well. The transient response of D2 shows a fast switching for 532, 633 and 851 nm wavelength excitation. As mentioned in the main text, the noise level for 532 and 633 nm wavelength excitation is found to be larger due to direct absorption in MoS<sub>2</sub>, which limits the minimum detectable power. However, for 851 nm excitation, like photodetector D1, we are able to detect an extremely low incident power. The responsivity values obtained for device D2 [Figure S1(d)] is comparable with the value obtained for detector D1, with the highest responsivity obtained being  $2.29 \times 10^6$  A/W. Figure S1(e) shows the calculated signal-to-noise ratio ( $SNR$ ) value as a function of illumination power falling on the detector. The extracted  $NEP$  is  $< 10.9 \text{ fW}/\sqrt{\text{Hz}}$  for 851 nm excitation.

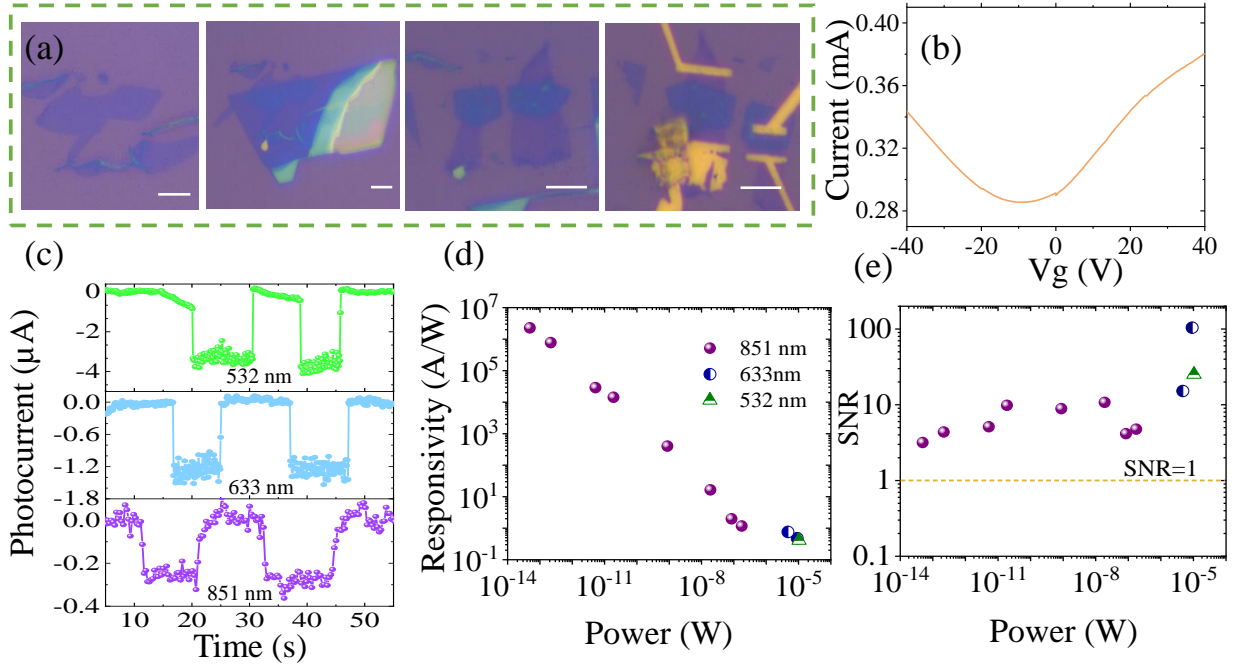

Figure S1: **Characterization of the device 2.** (a) Optical images at the different stages of fabrication of photodetector D2. Scale bar is 5  $\mu\text{m}$ . (b)  $I_d$ - $V_g$  characteristics for FLG under dark condition with  $V_d = 0.5$  V. (c) Temporal response of D2 at different wavelengths. The optical power incident on the device at 532, 633, and 851 nm are  $1.04 \times 10^{-5}$ ,  $4.72 \times 10^{-6}$ , and  $1.88 \times 10^{-11}$  W respectively. (d) Responsivity versus incident optical power at different excitation wavelengths. (e)  $SNR$  of the detector as a function of varying optical power.
